# Supplementary material for: DS-VLA: A Dendritic-inspired Vision-Language-Action Model for Robust Action Control
Source: arXiv:2609.32253 source file (2026-09-26)
Supplement: Supplementary file 1 [file appendix.tex]

\appendix

\section{A\quad Detailed Evaluation Protocol}

Input images are resized to $224\times224$, and the robot-state history contains 16 observations. Each episode begins with ten simulator-stabilization no-op steps that are excluded from the policy horizon. The maximum policy horizons are 220, 280, 300, and 520 steps for Spatial, Object, Goal, and Long, respectively. Predicted actions are mapped to the Franka execution space using the corresponding action de-normalization statistics.

Task success rate is
\begin{equation}
\mathrm{SR}
=\frac{N_{\mathrm{succ}}}{N_{\mathrm{all}}}\times100\%.
\end{equation}
We aggregate tasks within each suite and macro-average the four suite-level success rates.

All perturbations are applied to executed actions, while observations remain unchanged. Difficulty~1 perturbs policy steps 10--19 with translation and rotation Gaussian noise of standard deviation $0.1$ and $0.002$, respectively, and flips the gripper command. Difficulty~2 lasts 25 steps, uses translation/rotation noise of $0.010/0.004$, overwrites the first ten translation commands with $[0.50,0,0]$, and forces the gripper closed for 18 steps. Difficulty~3 lasts 35 steps, uses noise of $0.015/0.008$, overwrites the first 12 translation commands with $[0.65,-0.40,0]$, and forces closure for 25 steps. Overwrite vectors are commands in normalized policy-action space rather than Cartesian displacements.

\section{B\quad Action-Head Cost Derivation}

Let $T$ be the action horizon, $B$ the number of dendritic branches, $d_l$ and $h_l$ the input and output widths of layer $l$, $\widetilde d_l$ its branch-aligned input width, $\rho_l$ its firing rate, and $d_a$ the action dimension. The operations executed by the current dense DS-VLA implementation are
\begin{equation}
C_{\rm dense}^{\rm DS}
=T\left[
\sum_{l=1}^{L}(B+1)\widetilde d_lh_l
+h_Ld_a
\right].
\end{equation}
The $B+1$ factor includes the multi-branch dendritic projection and analog gate projection. Under ideal masked and event-driven execution, fixed zero mask entries are skipped and binary spikes trigger accumulations:
\begin{equation}
\begin{array}{l}
C_{\rm MAC}^{\rm DS}
=T\left[
\displaystyle\sum_{l=1}^{L}
(\widetilde d_lh_l+2Bh_l+2h_l)
+d_1h_1+h_Ld_a
\right],\\[2mm]
C_{\rm ACC}^{\rm DS}
=T\left[
\displaystyle\sum_{l=2}^{L}\rho_{l-1}d_lh_l
+\sum_{l=1}^{L}(2Bh_l+2h_l)
\right].
\end{array}
\end{equation}
The gate and the first dendritic projection remain MAC-based because they receive analog features. We estimate arithmetic energy as
\begin{equation}
E_{\rm arith}
=C_{\rm MAC}(\epsilon_{\rm mul}+\epsilon_{\rm add})
+C_{\rm ACC}\epsilon_{\rm add},
\end{equation}
where $\epsilon_{\rm mul}=3.1$\,pJ and $\epsilon_{\rm add}=0.1$\,pJ. The reported event-driven values assume firing rates of 0.10 and 0.05 at the two spike-driven transitions and are analytical estimates, not measured GPU energy.

For GPU measurements, the isolated native action heads are repeatedly executed after warm-up on an NVIDIA RTX~4090 at batch size one. OFT, DS-VLA, and GR00T are measured for 10,200, 300, and 100 iterations, respectively. Mean board energy per inference is computed as
\begin{equation}
E_{\rm board}
=P_{\rm avg}\,t_{\rm inference}.
\end{equation}
These measurements reflect the current dense PyTorch kernels. In particular, they do not realize zero-skipping or spike-triggered accumulation and therefore should not be interpreted as measurements of the ideal event-driven estimate.

\section{C\quad All-Model Analysis under Difficulty 1}

Table~\ref{tab:appendix_all_model_success} extends the main comparison by including DS-VLA without inhibitory gating. DS-VLA achieves the highest average success rate and leads on Goal, Spatial, and Long. It exceeds the ungated model by 20.9 percentage points on average, with gains of 22.0, 20.2, and 42.2 points on Goal, Spatial, and Long, respectively. The ungated model is 0.8 points higher on Object, but this isolated difference does not offset the large gains on the other suites.

\begin{table}[!ht]
\centering
\setlength{\tabcolsep}{0.7mm}
\begin{tabular}{lrrrrr}
\toprule
Model & Goal & Object & Spatial & Long & Avg. \\
\midrule
DS-VLA & \textbf{86.6} & 95.4 & \textbf{89.6} & \textbf{77.8} & \textbf{87.35} \\
OpenVLA-OFT & 54.4 & 21.8 & 80.4 & 1.2 & 39.45 \\
FAST & 27.4 & 13.8 & 54.4 & 0.0 & 23.90 \\
$\pi_0$ & 30.8 & 13.8 & 68.6 & 1.0 & 28.55 \\
GR00T & 31.8 & 30.4 & 60.8 & 0.0 & 30.75 \\
\shortstack[l]{DS-VLA without\\inhibitory gating} & 64.6 & \textbf{96.2} & 69.4 & 35.6 & 66.45 \\
\bottomrule
\end{tabular}
\caption{Success rate (\%) of all evaluated models under Difficulty~1.}
\label{tab:appendix_all_model_success}
\end{table}

The baseline failures are strongly suite dependent. OpenVLA-OFT remains relatively effective on Spatial but falls to 21.8\% on Object and 1.2\% on Long. FAST, $\pi_0$, and GR00T reach at most 30.75\% average success and nearly collapse on Long. In contrast, DS-VLA maintains at least 77.8\% on every suite, indicating that its robustness is not driven by one favorable task family.

Table~\ref{tab:appendix_cross_model} reports episode-level means over successful episodes. DS-VLA has inference latency and action variation comparable to the ungated dendritic SNN and to several VLA baselines. Its substantial success-rate gain therefore cannot be attributed to faster inference or simple output smoothing.

\begin{table}[!ht]
\centering
\setlength{\tabcolsep}{0.7mm}
\begin{tabular}{lrrrrrr}
\toprule
Model & Hor. & Hz & Inf. & Loop & $|A|$ & $|J|$ \\
\midrule
DS-VLA & 145.4 & 6.56 & 122.6 & 151.2 & .029 & .040 \\
OpenVLA-OFT & 117.5 & 9.91 & 68.1 & 98.9 & .026 & .029 \\
FAST & 126.4 & 2.07 & 454.9 & 486.8 & .070 & .122 \\
$\pi_0$ & 120.6 & 3.33 & 249.5 & 298.1 & .026 & .030 \\
GR00T & 120.3 & 6.71 & 116.9 & 147.4 & .028 & .037 \\
\shortstack[l]{DS-VLA w/o inhib.\\gating} & 142.5 & 6.38 & 127.7 & 155.5 & .027 & .038 \\
\bottomrule
\end{tabular}
\caption{Successful-trajectory statistics under Difficulty~1. Hor. is completion horizon; Inf. and Loop are in milliseconds.}
\label{tab:appendix_cross_model}
\end{table}

FAST exhibits the lowest action frequency and the largest action acceleration and jerk among its successful episodes, whereas OpenVLA-OFT has the lowest latency. However, these quantities must be interpreted jointly with success: each policy retains a different subset of episodes after failures are removed. The trajectory table therefore characterizes how successful recoveries are executed and should not be treated as an unconditional efficiency or smoothness ranking.

\section{D\quad Trajectory-Level Evaluation Details}

\subsection{Metric Definitions}

The main paper uses success rate as the primary robustness metric. The additional trajectory statistics below describe how successful episodes are executed and should not be interpreted as unconditional rankings across policies or perturbation levels. For a successful episode $e$ with $H_e$ policy steps, we report its completion horizon $H_e$, action frequency
\begin{equation}
f_e=\frac{H_e}{T_e^{\rm wall}},
\end{equation}
mean inference latency, and mean closed-loop latency. The closed-loop latency includes model inference and environment interaction for one policy update.

Let $a_t^{1:6}$ denote the six translation and rotation components of the predicted action at step $t$. Because these components are velocity-like control commands, the reported action acceleration and jerk are the element-wise absolute means of their first- and second-order finite differences:
\begin{equation}
\begin{array}{c}
\displaystyle
|A|_e=\frac{1}{6(H_e-1)}
\sum_{t=2}^{H_e}\left\|
\Delta a_t^{1:6}\right\|_1,\\[2mm]
\displaystyle
|J|_e=\frac{1}{6(H_e-2)}
\sum_{t=3}^{H_e}\left\|
\Delta^2 a_t^{1:6}\right\|_1.
\end{array}
\end{equation}
These quantities are computed in the normalized policy-action space and therefore should not be interpreted as physical Cartesian acceleration or jerk. Suite-level values are episode-level means over successful episodes only.

\subsection{Suite-Wise Successful-Trajectory Statistics}

Table~\ref{tab:appendix_success_horizon} reports the number of successful episodes, completion horizon, and action frequency for DS-VLA under the three perturbation difficulties. Each suite contains 500 evaluation episodes. Increasing difficulty generally increases the horizon of successful episodes, especially on Long, while action frequency remains in a narrow range.

\begin{table}[!ht]
\centering
\setlength{\tabcolsep}{1.0mm}
\begin{tabular}{llrrr}
\toprule
Suite & Level & Succ. & Hor. & Hz \\
\midrule
Goal    & D1 & 433 & 109.7 & 6.58 \\
Goal    & D2 & 363 & 122.0 & 6.38 \\
Goal    & D3 &  69 & 136.3 & 6.64 \\
Spatial & D1 & 448 & 100.5 & 6.29 \\
Spatial & D2 & 366 & 109.6 & 6.04 \\
Spatial & D3 & 248 & 123.2 & 6.39 \\
Object  & D1 & 477 & 134.8 & 6.72 \\
Object  & D2 & 448 & 150.7 & 6.80 \\
Object  & D3 & 378 & 155.0 & 6.93 \\
Long    & D1 & 389 & 250.0 & 6.64 \\
Long    & D2 & 256 & 275.1 & 6.89 \\
Long    & D3 & 225 & 279.2 & 6.80 \\
\bottomrule
\end{tabular}
\caption{Suite-wise DS-VLA statistics under increasing perturbation difficulty. Succ. is the number of successful episodes out of 500; Hor. and Hz are means over successful episodes.}
\label{tab:appendix_success_horizon}
\end{table}

Table~\ref{tab:appendix_timing_motion} reports timing and action-variation statistics for the same successful episodes. Inference and loop latency remain broadly stable as perturbation severity increases. The acceleration and jerk values similarly remain within a limited range, indicating that the increased completion horizon at higher difficulty is primarily associated with additional closed-loop interactions rather than a systematic increase in per-step computation.

\begin{table}[!ht]
\centering
\setlength{\tabcolsep}{0.8mm}
\begin{tabular}{llrrrr}
\toprule
Suite & Level & Inf. & Loop & $|A|$ & $|J|$ \\
\midrule
Goal    & D1 & 122.0 & 150.2 & .032 & .044 \\
Goal    & D2 & 126.8 & 155.2 & .027 & .038 \\
Goal    & D3 & 121.7 & 149.3 & .029 & .043 \\
Spatial & D1 & 121.8 & 156.6 & .034 & .044 \\
Spatial & D2 & 127.4 & 163.5 & .032 & .041 \\
Spatial & D3 & 120.8 & 154.8 & .036 & .049 \\
Object  & D1 & 122.3 & 147.7 & .027 & .039 \\
Object  & D2 & 120.5 & 146.1 & .025 & .035 \\
Object  & D3 & 118.0 & 143.7 & .025 & .035 \\
Long    & D1 & 124.6 & 150.2 & .023 & .032 \\
Long    & D2 & 120.3 & 144.9 & .022 & .031 \\
Long    & D3 & 121.7 & 146.6 & .023 & .033 \\
\bottomrule
\end{tabular}
\caption{Timing and action-variation statistics over successful DS-VLA episodes. Inf. and Loop are measured in milliseconds. $|A|$ and $|J|$ are computed from normalized translation and rotation action components.}
\label{tab:appendix_timing_motion}
\end{table}

\subsection{Interpretation}

Success-conditioned statistics have an inherent selection effect: as perturbations become more severe, the remaining successful trajectories may correspond to tasks or initial states that are easier to recover. Consequently, horizon, latency, acceleration, and jerk complement the success-rate results by describing the execution of recovered episodes, but they do not independently establish robustness, smoothness, or efficiency over all evaluation episodes.
